# Supplementary material for: Long-Horizon Planning with Latent World Models via Graph Anchors
Source: arXiv:2611.34509 source file (2026-12-01)
Supplement: Supplementary file 1 [file supp_labels.tex]

% generated by figs/scripts/export_labels.py from supp.aux; do not edit
\newlabel{app:phenomenon}{{A}{2}{}{}{}}
\newlabel{app:phenomenon@cref}{{[section][1][]A}{[1][2][]2}{}{}{}}
\newlabel{app:falls}{{A}{2}{}{}{}}
\newlabel{app:falls@cref}{{[section][1][]A}{[1][2][]2}{}{}{}}
\newlabel{app:published}{{A}{2}{}{}{}}
\newlabel{app:published@cref}{{[section][1][]A}{[1][2][]2}{}{}{}}
\newlabel{app:search}{{A}{2}{}{}{}}
\newlabel{app:search@cref}{{[section][1][]A}{[1][2][]2}{}{}{}}
\newlabel{app:closedloop}{{A}{2}{}{}{}}
\newlabel{app:closedloop@cref}{{[section][1][]A}{[1][2][]2}{}{}{}}
\newlabel{tab:published}{{S1}{2}{}{}{}}
\newlabel{tab:published@cref}{{[table][1][]S1}{[1][2][]2}{}{}{}}
\newlabel{app:graphs}{{B}{2}{}{}{}}
\newlabel{app:graphs@cref}{{[section][2][]B}{[1][2][]2}{}{}{}}
\newlabel{app:ranktest}{{B.1}{2}{}{}{}}
\newlabel{app:ranktest@cref}{{[subsection][1][2]B.1}{[1][2][]2}{}{}{}}
\newlabel{app:range}{{B.1}{2}{}{}{}}
\newlabel{app:range@cref}{{[subsection][1][2]B.1}{[1][2][]2}{}{}{}}
\newlabel{fig:e1range}{{S1}{3}{}{}{}}
\newlabel{fig:e1range@cref}{{[figure][1][]S1}{[1][3][]3}{}{}{}}
\newlabel{app:epochs}{{B.2}{3}{}{}{}}
\newlabel{app:epochs@cref}{{[subsection][2][2]B.2}{[1][3][]3}{}{}{}}
\newlabel{app:checks}{{B.3}{3}{}{}{}}
\newlabel{app:checks@cref}{{[subsection][3][2]B.3}{[1][3][]3}{}{}{}}
\newlabel{tab:truediag}{{S2}{3}{}{}{}}
\newlabel{tab:truediag@cref}{{[table][2][]S2}{[1][3][]3}{}{}{}}
\newlabel{fig:e1maps}{{S2}{4}{}{}{}}
\newlabel{fig:e1maps@cref}{{[figure][2][]S2}{[1][3][]4}{}{}{}}
\newlabel{fig:e2epochs}{{S3}{4}{}{}{}}
\newlabel{fig:e2epochs@cref}{{[figure][3][]S3}{[1][3][]4}{}{}{}}
\newlabel{app:theory}{{B.4}{5}{}{}{}}
\newlabel{app:theory@cref}{{[subsection][4][2]B.4}{[1][5][]5}{}{}{}}
\newlabel{lem:transfer}{{1}{5}{}{}{}}
\newlabel{lem:transfer@cref}{{[lemma][1][]1}{[1][5][]5}{}{}{}}
\newlabel{cor:true}{{1}{5}{}{}{}}
\newlabel{cor:true@cref}{{[corollary][1][]1}{[1][5][]5}{}{}{}}
\newlabel{prop:drift}{{1}{5}{}{}{}}
\newlabel{prop:drift@cref}{{[proposition][1][]1}{[1][5][]5}{}{}{}}
\newlabel{fig:diag}{{S4}{6}{}{}{}}
\newlabel{fig:diag@cref}{{[figure][4][]S4}{[1][5][]6}{}{}{}}
\newlabel{fig:hops}{{S5}{6}{}{}{}}
\newlabel{fig:hops@cref}{{[figure][5][]S5}{[1][5][]6}{}{}{}}
\newlabel{tab:driftt8}{{S3}{6}{}{}{}}
\newlabel{tab:driftt8@cref}{{[table][3][]S3}{[1][6][]6}{}{}{}}
\newlabel{app:predicts}{{B.5}{6}{}{}{}}
\newlabel{app:predicts@cref}{{[subsection][5][2]B.5}{[1][6][]6}{}{}{}}
\newlabel{app:focusmain}{{C}{7}{}{}{}}
\newlabel{app:focusmain@cref}{{[section][3][]C}{[1][7][]7}{}{}{}}
\newlabel{app:focus}{{C.1}{7}{}{}{}}
\newlabel{app:focus@cref}{{[subsection][1][3]C.1}{[1][7][]7}{}{}{}}
\newlabel{app:pushbias}{{C.2}{7}{}{}{}}
\newlabel{app:pushbias@cref}{{[subsection][2][3]C.2}{[1][7][]7}{}{}{}}
\newlabel{app:remedy}{{D}{7}{}{}{}}
\newlabel{app:remedy@cref}{{[section][4][]D}{[1][7][]7}{}{}{}}
\newlabel{app:remedyproof}{{D.1}{7}{}{}{}}
\newlabel{app:remedyproof@cref}{{[subsection][1][4]D.1}{[1][7][]7}{}{}{}}
\newlabel{fig:theory}{{S6}{8}{}{}{}}
\newlabel{fig:theory@cref}{{[figure][6][]S6}{[1][7][]8}{}{}{}}
\newlabel{app:method}{{D.2}{8}{}{}{}}
\newlabel{app:method@cref}{{[subsection][2][4]D.2}{[1][8][]8}{}{}{}}
\newlabel{alg:sga}{{S1}{8}{}{}{}}
\newlabel{alg:sga@cref}{{[algorithm][1][]S1}{[1][8][]8}{}{}{}}
\newlabel{alg:graph}{{S1}{8}{}{}{}}
\newlabel{alg:graph@cref}{{[algorithm][1][]S1}{[1][8][]8}{}{}{}}
\newlabel{alg:anchor}{{S1}{8}{}{}{}}
\newlabel{alg:anchor@cref}{{[algorithm][1][]S1}{[1][8][]8}{}{}{}}
\newlabel{alg:plan}{{S1}{8}{}{}{}}
\newlabel{alg:plan@cref}{{[algorithm][1][]S1}{[1][8][]8}{}{}{}}
\newlabel{fig:e1hops}{{S7}{9}{}{}{}}
\newlabel{fig:e1hops@cref}{{[figure][7][]S7}{[1][7][]9}{}{}{}}
\newlabel{tab:mw}{{S4}{10}{}{}{}}
\newlabel{tab:mw@cref}{{[table][4][]S4}{[1][8][]10}{}{}{}}
\newlabel{fig:exchange}{{S8}{10}{}{}{}}
\newlabel{fig:exchange@cref}{{[figure][8][]S8}{[1][7][]10}{}{}{}}
\newlabel{app:impl}{{D.3}{10}{}{}{}}
\newlabel{app:impl@cref}{{[subsection][3][4]D.3}{[1][10][]10}{}{}{}}
\newlabel{fig:suppgraph}{{S9}{11}{}{}{}}
\newlabel{fig:suppgraph@cref}{{[figure][9][]S9}{[1][8][]11}{}{}{}}
\newlabel{fig:suppanchor}{{S10}{11}{}{}{}}
\newlabel{fig:suppanchor@cref}{{[figure][10][]S10}{[1][8][]11}{}{}{}}
\newlabel{fig:suppcost}{{S11}{12}{}{}{}}
\newlabel{fig:suppcost@cref}{{[figure][11][]S11}{[1][10][]12}{}{}{}}
\newlabel{tab:graphs}{{S5}{12}{}{}{}}
\newlabel{tab:graphs@cref}{{[table][5][]S5}{[1][12][]12}{}{}{}}
\newlabel{app:results}{{E}{12}{}{}{}}
\newlabel{app:results@cref}{{[section][5][]E}{[1][12][]12}{}{}{}}
\newlabel{app:seeds}{{E.1}{12}{}{}{}}
\newlabel{app:seeds@cref}{{[subsection][1][5]E.1}{[1][12][]12}{}{}{}}
\newlabel{app:retrain}{{E.1}{12}{}{}{}}
\newlabel{app:retrain@cref}{{[subsection][1][5]E.1}{[1][12][]12}{}{}{}}
\newlabel{app:stats}{{E.1}{12}{}{}{}}
\newlabel{app:stats@cref}{{[subsection][1][5]E.1}{[1][12][]12}{}{}{}}
\newlabel{app:handoff}{{E.2}{12}{}{}{}}
\newlabel{app:handoff@cref}{{[subsection][2][5]E.2}{[1][12][]12}{}{}{}}
\newlabel{tab:compare}{{S6}{13}{}{}{}}
\newlabel{tab:compare@cref}{{[table][6][]S6}{[1][12][]13}{}{}{}}
\newlabel{fig:suppoptions}{{S12}{14}{}{}{}}
\newlabel{fig:suppoptions@cref}{{[figure][12][]S12}{[1][12][]14}{}{}{}}
\newlabel{tab:retrain}{{S7}{14}{}{}{}}
\newlabel{tab:retrain@cref}{{[table][7][]S7}{[1][12][]14}{}{}{}}
\newlabel{app:contactcfg}{{E.2}{14}{}{}{}}
\newlabel{app:contactcfg@cref}{{[subsection][2][5]E.2}{[1][14][]14}{}{}{}}
\newlabel{fig:plannerviewpusht}{{S13}{14}{}{}{}}
\newlabel{fig:plannerviewpusht@cref}{{[figure][13][]S13}{[1][14][]14}{}{}{}}
\newlabel{tab:contactcfg}{{S8}{14}{}{}{}}
\newlabel{tab:contactcfg@cref}{{[table][8][]S8}{[1][14][]14}{}{}{}}
\newlabel{app:ablations}{{E.3}{14}{}{}{}}
\newlabel{app:ablations@cref}{{[subsection][3][5]E.3}{[1][14][]14}{}{}{}}
\newlabel{fig:ablate}{{S14}{15}{}{}{}}
\newlabel{fig:ablate@cref}{{[figure][14][]S14}{[1][14][]15}{}{}{}}
\newlabel{tab:factorial}{{S9}{15}{}{}{}}
\newlabel{tab:factorial@cref}{{[table][9][]S9}{[1][15][]15}{}{}{}}
\newlabel{tab:search}{{S9}{15}{}{}{}}
\newlabel{tab:search@cref}{{[table][9][]S9}{[1][15][]15}{}{}{}}
\newlabel{tab:spanh}{{S10}{15}{}{}{}}
\newlabel{tab:spanh@cref}{{[table][10][]S10}{[1][15][]15}{}{}{}}
\newlabel{tab:stress}{{S11}{15}{}{}{}}
\newlabel{tab:stress@cref}{{[table][11][]S11}{[1][15][]15}{}{}{}}
\newlabel{app:beyond}{{E.4}{15}{}{}{}}
\newlabel{app:beyond@cref}{{[subsection][4][5]E.4}{[1][15][]15}{}{}{}}
\newlabel{fig:robust}{{S15}{16}{}{}{}}
\newlabel{fig:robust@cref}{{[figure][15][]S15}{[1][15][]16}{}{}{}}
\newlabel{app:baselines}{{E.5}{16}{}{}{}}
\newlabel{app:baselines@cref}{{[subsection][5][5]E.5}{[1][16][]16}{}{}{}}
\newlabel{tab:dwmcost}{{S12}{16}{}{}{}}
\newlabel{tab:dwmcost@cref}{{[table][12][]S12}{[1][16][]16}{}{}{}}
\newlabel{app:contemp}{{E.6}{17}{}{}{}}
\newlabel{app:contemp@cref}{{[subsection][6][5]E.6}{[1][17][]17}{}{}{}}
\newlabel{fig:pushtdist}{{S16}{17}{}{}{}}
\newlabel{fig:pushtdist@cref}{{[figure][16][]S16}{[1][17][]17}{}{}{}}
\newlabel{tab:pldm}{{S13}{18}{}{}{}}
\newlabel{tab:pldm@cref}{{[table][13][]S13}{[1][17][]18}{}{}{}}
\newlabel{tab:budget}{{S13}{18}{}{}{}}
\newlabel{tab:budget@cref}{{[table][13][]S13}{[1][17][]18}{}{}{}}
\newlabel{tab:graphpol}{{S14}{18}{}{}{}}
\newlabel{tab:graphpol@cref}{{[table][14][]S14}{[1][17][]18}{}{}{}}
\newlabel{tab:waypoint2}{{S14}{18}{}{}{}}
\newlabel{tab:waypoint2@cref}{{[table][14][]S14}{[1][17][]18}{}{}{}}
\newlabel{tab:contemp}{{S15}{19}{}{}{}}
\newlabel{tab:contemp@cref}{{[table][15][]S15}{[1][17][]19}{}{}{}}
\newlabel{tab:fidelity}{{S15}{19}{}{}{}}
\newlabel{tab:fidelity@cref}{{[table][15][]S15}{[1][17][]19}{}{}{}}
\newlabel{tab:metrosweep}{{S16}{19}{}{}{}}
\newlabel{tab:metrosweep@cref}{{[table][16][]S16}{[1][18][]19}{}{}{}}
\newlabel{tab:apoffset}{{S16}{19}{}{}{}}
\newlabel{tab:apoffset@cref}{{[table][16][]S16}{[1][18][]19}{}{}{}}
\newlabel{tab:comp_mech}{{S17}{20}{}{}{}}
\newlabel{tab:comp_mech@cref}{{[table][17][]S17}{[1][18][]20}{}{}{}}
\newlabel{tab:exec}{{S18}{21}{}{}{}}
\newlabel{tab:exec@cref}{{[table][18][]S18}{[1][21][]21}{}{}{}}
\newlabel{app:repro}{{E.7}{21}{}{}{}}
\newlabel{app:repro@cref}{{[subsection][7][5]E.7}{[1][21][]21}{}{}{}}
\newlabel{app:limits}{{F}{21}{}{}{}}
\newlabel{app:limits@cref}{{[section][6][]F}{[1][21][]21}{}{}{}}
\newlabel{fig:compquant}{{S17}{22}{}{}{}}
\newlabel{fig:compquant@cref}{{[figure][17][]S17}{[1][21][]22}{}{}{}}
\newlabel{app:qual}{{F.2}{22}{}{}{}}
\newlabel{app:qual@cref}{{[subsection][2][6]F.2}{[1][22][]22}{}{}{}}
\newlabel{fig:companatomy}{{S18}{23}{}{}{}}
\newlabel{fig:companatomy@cref}{{[figure][18][]S18}{[1][21][]23}{}{}{}}
\newlabel{fig:qual}{{S19}{24}{}{}{}}
\newlabel{fig:qual@cref}{{[figure][19][]S19}{[1][21][]24}{}{}{}}
\newlabel{fig:plannerview}{{S20}{24}{}{}{}}
\newlabel{fig:plannerview@cref}{{[figure][20][]S20}{[1][22][]24}{}{}{}}
\newlabel{tab:seedsx}{{S19}{25}{}{}{}}
\newlabel{tab:seedsx@cref}{{[table][19][]S19}{[1][21][]25}{}{}{}}
